# Supplementary material for: WeaNF: Weak Supervision with Normalizing Flows
Source: arXiv:2204.13409 source file (2022-05-02)
Supplement: Supplementary file 1 [file appendix_more_examples.tex]

\section{More Examples}
\label{sec:app_more_examples}

\begin{table*}
\centering
\small
\begin{tabular}{llllrr}
\toprule
 rule & example & $P( \lambda | x)$  & Label $(\lambda)$ & Gold label  &  Prediction \\
\midrule
*boring* & ... take a nap ... &  & 0 & 0 & 0 \\
(won) .* (claim)  & you've won tkts to ..  euro final ..  collect ..& NoN & spam & spam & spam\\
(miss) .* (you) & ..  tot about u 2day.love n miss.take care.	& NoN & no spam & ns & ns \\
(what) .* (year | hour |...)& What is Susan B. Anthony 's birthday ?  & NoN & NUM & NUM & NUM \\
how .* (much|many) & How many admirals ... Navy? & 1 & NUM &  NUM & NUM \\ % rule 29
Who .* & Which US president ... ? & 1 & PER & PER & PER \\ % rule 20
\bottomrule
\end{tabular}

\caption{We inspect some labelling functions (with semantic meaning) and choose some selected example from the $10$ most likely or unlikely probabilities $P(x| \lambda)$.  Here, we look at the standard model. Note that the rules are simplified and the texts are shortened, as the examples wouldn't fit.  See Appendix for the full examples. %TODO
for the full rules.}
\label{table:examples}
\end{table*}
